# Supplementary material for: Probabilistic Modelling is Sufficient for Causal Inference
Source: arXiv:2512.23408 source file (2025-12-29)
Supplement: Supplementary file 1 [file counterfactual-intro-appendix.tex]

% What are interventions
Interventional questions can be seen as ones that seek to infer the hypothetical effects of a contemplated manipulation in a system. These correspond to questions like: ``What's the effectiveness of aspirin on reducing headache duration?'', ``How would changing regulations on cigarette companies impact population's life-expectancy?'', or ``How effective is a lock-down at suppressing the spread of a pandemic?'' % Maybe cite the paper

% A different kind of problem -- counterfactuals
A different type of questions we might also want to ask is about what might have happened in previously observed cases had something been done differently. What would have happened in the case of the specific person/example/instance at hand in an alternative world, were some values and/or mechanisms in our model altered? Some examples of such \emph{counterfactual} questions would be: ``Would I still have a headache now had I taken a larger dose of aspirin?'', or ``How many disease cases would there be in the population of country that didn't implement lock-down, had a lock-down not been put in place?''

% \footnotetext{This latter counterfactual question and the question about the effectiveness of non-pharmaceutical interventions on pandemic spread have been addressed in the context of COVID-19 by Flaxman et al. \cite{flaxman2020report}.}%, Mishra and Gandy et al. \cite{flaxman2020report}.}

% CF relevant in legal
Counterfactual analysis can be used when trying to assign blame for an outcome, or when assessing the cause of an event \citep{pearl2015causes}. This bears significance in, for instance, legal fields, where the court may seek to assign responsibility for something that has happened \citep{dawid2014fittingscience}. For example, a judge might wish to conclude that ``were it not for the defendant's actions, the chemical spill would in all likelihood not have occurred''. With probabilistic modelling, we can endeavour to quantify how likely or unlikely different outcomes would have been had different actions been taken. 

% How could we model what would have happened?
Intuitively, when talking about things that might have happened had some factor been different, we might consider a hypothetical world that is the same as the observed one, with the exception of the alteration of interest. A common expression in economics for this line of thinking is \textit{ceteris paribus} --- `all other things being equal'. Stating \textit{ceteris paribus} as an assumption, however, is fairly ambiguous in itself. We might prefer to specify what exactly is being held equal and what isn't \citet[\textsection7.2.2]{pearl2000causality}.
One way to do so with probabilistic modelling is to share the desired variables between two settings --- the observed and the counterfactual --- making modelling assumptions explicit.
One can state such assumptions implicitly with a shorthand by specifying a \textit{Structural Causal Model} \citep{peters2017elements,pearl2000causality}, and obtaining the joint distribution over all settings of interest implicitly from it.
